# Supplementary material for: Hydrodynamics in Semidilute Polyelectrolyte Solutions and Complex Coacervates
Source: arXiv:2409.09450 source file (2024-09-14)
Supplement: Supplementary file 1 [file Hydrodynamcis_SI.pdf]

# Supplemental Material for
# Hydrodynamics in Semidilute Polyelectrolyte Solutions and Complex Coacervates

Shensheng Chen and Zhen-Gang Wang*
*Division of Chemistry and Chemical Engineering,*
*California Institute of Technology, Pasadena, CA 91125*

## A. Other simulation details

In our GCMe simulations, the reduced number density is set to $\rho = 2.5$, and the integration time step is $\delta t = 0.02\tau$, which are the default setup in the original method development [1]. All simulations are run in the canonical (NVT) ensemble, with the first $10^5$ steps for equilibration, followed by $10^7$ steps for production. The long-range electrostatics is solved by the Particle-Particle-Particle-Mesh (PPPM) algorithm with a precision of $10^{-4}$. The overlap concentration $c^*$ for PE solutions is determined by gradually increasing the number of chains in the simulation box until the pervaded volume of all chains reaches 64% of the simulation box [2]. For $N = 100$, the overlap concentration corresponds to about 18 chains (out of a total number of 540,000 particles). For the coacervate systems, the charge fraction of both polycation and polyanion is set to $f = 1/3$ with charged beads evenly distributed along the PE chains. All the simulations are performed using the LAMMPS platform [3].

## B. Structure factor, correlation length, intermediate scattering function, and chain diffusion

To evaluate the collective dynamics of the polymers, we calculate the intermediate scattering function $F(q,t)$ of all $N_t$ polymer beads as

$$F(\boldsymbol{q},t) = \frac{1}{N_t}\sum_{\alpha=1}^{N_t}\sum_{\beta=1}^{N_t}\langle \exp[i\boldsymbol{q}\cdot(\boldsymbol{r}_\alpha(t) - \boldsymbol{r}_\beta(0))]\rangle \qquad (1)$$

where $\boldsymbol{q}$ is the wavevector. When $t = 0$, the intermediate scattering function reduces to the static structure factor $S(q) = F(q,0)$.

Figure S1(a) shows the static structure factor $S(q)$ of semidilute PE solutions with chain length $N = 100$ at different polymer concentrations $c/c^*$ . All systems show a peak at $q_\xi$. The length scale at the peak of the structure factor is the correlation length given by $\xi = 2\pi/q_\xi$. Figure S1(b) shows the wavenumber at structure peak scales with the polymer concentration as $q_\xi \sim c^{1/2}$, in agreement with theoretical predictions [4, 5]. From collective dynamics, we obtain the relaxation time $\tau_{re}$ by

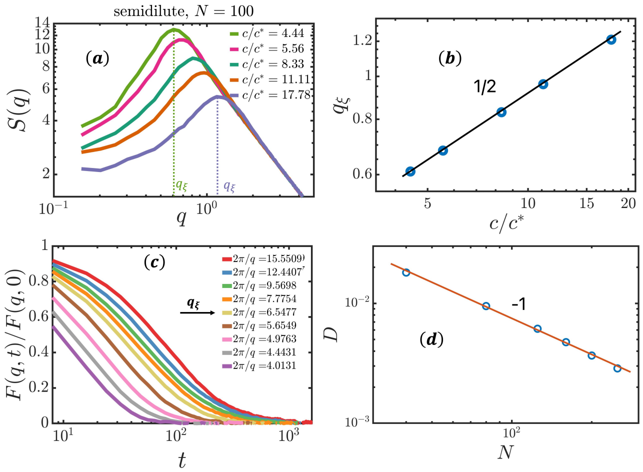


FIG. S1. (a) Static structure factor of semidilute PE solutions with chain length $N = 100$ at different concentrations. The dashed lines mark the positions of the structure peaks $q_\xi$ (b) The wavenumber at the structure peak as a function of polymer concentration for semidilute PE solutions. (c) Intermediate scattering function for several $q$ values, for a system with $N = 100$ at $c/c^* = 11.1$. (d) Chain center-of-mass diffusivity with different chain lengths at a fixed polymer concentration $c/c^* = 11.1$ for the semidilute PE solution.

fitting the normalized intermediate scattering function into a stretched exponential decay

$$F(q,t)/F(q,0) = \exp[-(t/\tau_{re})^\beta] \qquad (2)$$

For the data presented in the main text, $\beta$ falls in the range $0.76 \sim 0.97$ and $0.62 \sim 0.93$, respectively, for semidilute PE solution systems and PE coacervate systems, with the relaxation for larger $q$ having a $\beta$ closer to 1. Figure S1(c) shows the decay of $F(q,t)/F(q,0)$ in a semidilute PE solution for several values of $q$. The top few curves in the figure are found to not fit will with the simple stretched exponential decay, indicating the relevant dynamics has a multimode character, which may be related to the unresolved “slow mode” controversy [6, 7]. For this reason, we only report the relaxation time for $q > q_\xi$ in the main text for semidilute PE solutions.

Figure S1(d) shows the chain center-of-mass diffusivity as a function of chain length in semidilute PE solutions at a fixed polymer concentration $c/c^* = 11.1$. The diffusivity scales with chain length as $D \sim N^{-1}$, consistent with theoretical predictions [4, 5, 8, 9].

* zgw@caltech.edu

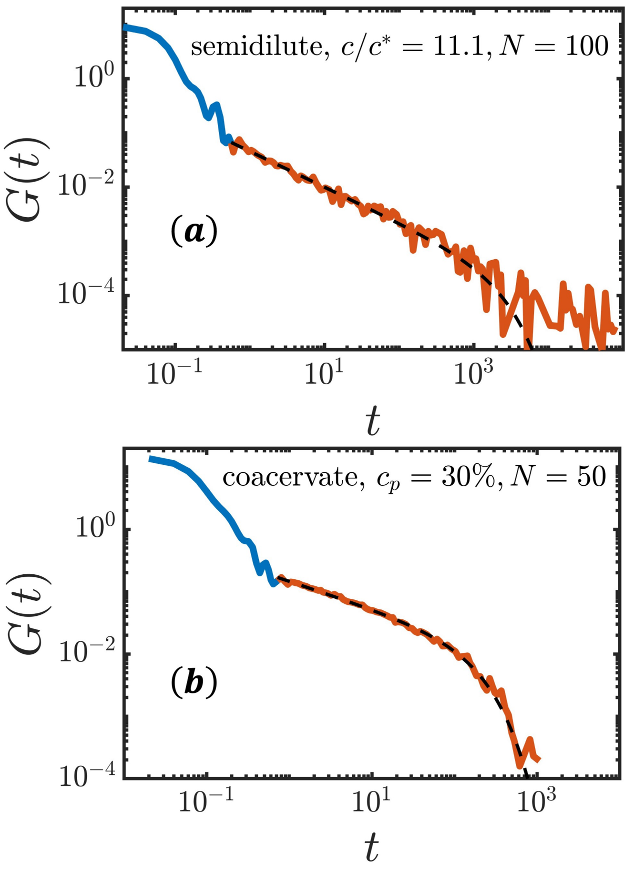


FIG. S2. Stress relaxation function $G(t)$ for (a) a semidilute PE solution with chain length $N = 100$ atconcentration $c/c^* = 11.1$; and (b) a PE complex coacervate with $N = 50$ at total polymer concentration 30%. The dash lines are the fittings to the red portion of the simulation data.

### C. Rheological response

To obtain the $G'$ and $G''$, we first calculate the stress relaxation function [10] as $G(t) = \frac{V}{5k_BT}\left[\langle\sigma_{xy}(t)\sigma_{xy}(0)\rangle + \langle\sigma_{xz}(t)\sigma_{xz}(0)\rangle + \langle\sigma_{yz}(t)\sigma_{yz}(0)\rangle\right] + \frac{V}{30k_BT}\left[\langle I_{xy}(t)I_{xy}(0)\rangle + \langle I_{xz}(t)I_{xz}(0)\rangle + \langle I_{yz}(t)I_{yz}(0)\rangle\right]$ on the fly in the simulation via a "multi-tau" algorithm [11] implemented in LAMMPS. Here $\sigma_{\alpha\beta}$ is the stress tensor in the $\alpha$ and $\beta$ directions, and $I_{\alpha\beta} = \sigma_{\alpha\alpha} - \sigma_{\beta\beta}$. $G'$ and $G''$ are then calculated from the sine and cosine Fourier transform of $G(t)$, as

$$G'(\omega) = \omega \int_0^\infty G(t)\sin(\omega t)dt \tag{3}$$

and

$$G''(\omega) = \omega \int_0^\infty G(t)\cos(\omega t)dt \tag{4}$$

The results of $G(t)$ for a semidilute PE solution and a complex coacervate are shown in Fig. S2. In practice, since $G(t)$ become noisy (and can become negative) at later times, we fit $G(t)$ to a suggested analytical expression [12] $G(t) = a * \left(\frac{t}{t_0}\right)^b * \exp(-\frac{t}{\tau_0})$ for data after $t_0$ before performing the Fourier transform, with $a = 0.16, t_0 = 0.14$ for the semidilute PE solution and $a = 0.26, t_0 = 0.28$ for the complex coacervate shown in Fig. S2. The fitting parameters are $b = 0.65, \tau_0 = 2724$ and $b = 0.44, \tau = 175.6$ for the two systems, respectively.


[1] B. B. Ye, S. Chen, and Z.-G. Wang, GCMe: Efficient Implementation of the Gaussian Core Model with Smeared Electrostatic Interactions for Molecular Dynamics Simulations of Soft Matter Systems, Journal of Chemical Theory and Computation 10.1021/acs.jctc.4c00603 (2024).

[2] J. A. Bollinger, G. S. Grest, M. J. Stevens, and M. Rubinstein, Overlap Concentration in Salt-Free Polyelectrolyte Solutions, Macromolecules **54**, 10068 (2021).

[3] A. P. Thompson, H. M. Aktulga, R. Berger, D. S. Bolintineanu, W. M. Brown, P. S. Crozier, P. J. in 't Veld, A. Kohlmeyer, S. G. Moore, T. D. Nguyen, R. Shan, M. J. Stevens, J. Tranchida, C. Trott, and S. J. Plimpton, LAMMPS - a flexible simulation tool for particle-based materials modeling at the atomic, meso, and continuum scales, Computer Physics Communications **271**, 108171 (2022).

[4] M. Rubinstein, R. H. Colby, and A. V. Dobrynin, Dynamics of Semidilute Polyelectrolyte Solutions, Physical Review Letters **73**, 2776 (1994).

[5] A. V. Dobrynin, R. H. Colby, and M. Rubinstein, Scaling Theory of Polyelectrolyte Solutions, Macromolecules **28**, 1859 (1995).

[6] M. Sedlák and E. J. Amis, Dynamics of moderately concentrated salt-free polyelectrolyte solutions: Molecular weight dependence, The Journal of Chemical Physics **96**, 817 (1992).

[7] M. Sedlák, The ionic strength dependence of the structure and dynamics of polyelectrolyte solutions as seen by light scattering: The slow mode dilemma, The Journal of Chemical Physics **105**, 10123 (1996).

[8] R. H. Colby, Structure and linear viscoelasticity of flexible polymer solutions: comparison of polyelectrolyte and neutral polymer solutions, Rheologica Acta **49**, 425 (2010).

[9] M. Muthukumar, Dynamics of polyelectrolyte solutions, The Journal of Chemical Physics **107**, 2619 (1997).

[10] P. J. Daivis and D. J. Evans, Comparison of constant pressure and constant volume nonequilibrium simulations of sheared model decane, The Journal of Chemical Physics **100**, 541 (1994).

[11] J. Ramírez, S. K. Sukumaran, B. Vorselaars, and A. E. Likhtman, Efficient on the fly calculation of time correlation functions in computer simulations, The Journal of Chemical Physics **133**, 154103 (2010).

[12] M. Rubinstein and R. H. Colby, *Polymer Physics* (Oxford University PressOxford, 2003).
